# Supplementary material for: Conditional Encryption with Applications to Secure Personalized Password Typo Correction
Source: arXiv:2409.06128 source file (2026-03-21)
Supplement: Supplementary file 1 [file ArtifactAppendix.tex]

\section{Artifact Appendix}

\emph{The Artifact Appendix is meant to summarize the purpose,
availability, content, dependencies, and execution of the artifacts
that support your paper.  It should include a clear description of
your artifacts' hardware, software, and configuration requirements.
If your artifacts have received the \emph{Artifacts
Evaluated--Functional}, \emph{Artifacts Evaluated--Reusable}, or
\emph{Results Reproduced} badge, this appendix should summarize the
relevant major claims made by your paper and provide instructions for
validating each claim through the use of your artifacts.  Linking the
claims of your paper to the artifacts allows a reader of your paper
to more easily try to reproduce your paper's results.}

\emph{Please fill in all the mandatory sections, keeping their titles
and organization but removing the current illustrative content, and
remove the optional sections that do not apply to your artifacts.}

%%%%%%%%%%%%%%%%%%%%%%%%%%%%%%%%%%%%%%%%%%%%%%%%%%%%%%%%%%%%%%%%%%%%%

\subsection{Abstract}

\emph{[Mandatory]}
In this artifact, we describe the procedure for installing and implementing our proposed conditional encryption scheme, as well as the conditional TypTop (CondTypTop) system. The artifact is divided into two main sections: one focused on conditional encryption, and the other on CondTypTop, which is the TypTop system implemented using conditional encryption as its core building block. For each section, we provide detailed steps for installing, compiling the C++ implementation, and running basic functionality tests. Additionally, we include instructions for evaluating the performance of each part—conditional encryption and CondTypTop—by reproducing the results presented in \figref{fig:FullEvalCondEnc} and the data shown in \tableref{CondEncEmp} and \tableref{CondTypComp}. 
We provide a link to the detailed README.md file, which explains how to install the artifact, run basic tests, and evaluate performance. To simplify the artifact review process, we have included several ``$\mathtt{*.sh}$'' scripts that can be executed to generate the desired outputs by calling the functions contained in the compiled  c++ codes. In the README.md file, we describe the expected output for each test case, which can be verified by running the provided scripts. Additionally, we offer instructions on how to obtain different results by executing the scripts with various arguments.

% \emph{Provide a short description of your artifacts.  What do they
% contain?  How are they packaged?  What do they do when executed?  What
% results to they produce?  How are your artifacts licensed?  Be brief;
% subsequent sections of this appendix can be used fill in the details.}

%%%%%%%%%%%%%%%%%%%%%%%%%%%%%%%%%%%%%%%%%%%%%%%%%%%%%%%%%%%%%%%%%%%%%

\subsection{Description \& Requirements}
The experiments in this artifact were conducted on a Lenovo ThinkStation S30 with a $2.9$ GHz 8-core Intel\textsuperscript{\textregistered} Xeon\textsuperscript{\textregistered} E5-26900x 16 CPU processor (16 cores) and $28$ GiB of DDR4 RAM memory, and 1.0 TB disk. The system runs on Ubuntu 24.04 LTS with GNOME version 46 and uses the Wayland windowing system. The kernel version is Linux 6.8.0-41-generic. For those wishing to recreate the experimental environment, the minimum hardware requirements are a multi-core processor (at least 8 cores recommended) and 16 GiB of RAM. The software requirements include a 64-bit Linux distribution, preferably Ubuntu 20.04 LTS or later, with support for GNOME and Wayland, as well as the following development tools:
\begin{itemize}
    \item C++ compiler (g++)
    \item CMake (version 3.18 or later)
    \item Make (for compiling and building)
\end{itemize}

All scripts in the artifact rely on a Linux-based environment with access to these tools.

Benchmarks included in the artifact, executed via provided shell scripts, assess both performance and correctness. Detailed instructions for compiling the C++ code and running the performance tests are included in the README.md file.

% \emph{This section should further detail your artifacts and summarize
% the requirements that must be met for a person to recreate an
% experimental environment for utilizing your artifacts.  Where
% applicable, state the minimum hardware and software requirements for
% running your artifacts.  It is also good practice to list and describe
% in this section benchmarks where those are part of, or simply have
% been used to produce results with, your artifacts.}

\emph{[Mandatory]}
The artifact is organized into several key directories and files, as can be seen in the directory of the downloaded files from Zenodo. Here is a general road map to help navigate through them:
\begin{itemize}
    \item \textbf{README.md}: This file provides a detailed description of how to install, compile, and run the various components of the project. It also includes instructions for running tests and performance evaluations. Start here for setup instructions and usage information. This file also provide some example test case and its corresponding output. 

    \item \textbf{src}: This directory contains the core source code, including the implementations of the cryptographic functions and conditional encryption schemes discussed in the paper. Specifically, it includes:
    \begin{itemize}
        \item Cryptowrapper functions.
        \item Paillier wrapper functions.
        \item Conditional encryption \item Implementations for various predicates such as Hamming distance, Edit distance, CAPSLOCK\_ON and OR\_of \_CAPSLOCK \_EditDist1\_HamDist2 (Typo predicate). 
    \end{itemize}

    \item \textbf{test}: This directory includes the test files and datasets used for evaluating the performance of our suggested conditional encryption schemes. The PWDVsTypoDataSet is particularly important, as it contains the random input data (pair of PWD and their typos collected from Chaterjee data set and filtered under different limitation like PWD size, hamming and edit distance, etc) fed into the conditional encryption algorithms during testing.

    \item \textbf{CMakeLists.txt}: This file handles the configuration of the project and facilitates the build process. It copies necessary scripts, such as TestScript.sh, to the build/test directory. This script is used to run the compiled test binaries and is critical for generating data for performance evaluations and experiments (e.g., plotting results for Figure 1.a).

    \item \textbf{GeneratePlotsPdfs}: This directory contains the necessary scripts and tools for plotting the results of the experiments. The CMakeLists.txt file copies this directory to the test directory, where it reads the generated ``*.dat'' files to produce PDF output of the experiment results. For this part, we assume that the the machine include Latex compiling software like pdflatex.
    
    \item \textbf{Third-party Libraries}: 
    \begin{itemize}
        \item argon2/phcargon2: This folder contains the implementation of Argon2, a memory-hard function used in the project
        \item paillier: This directory includes the Paillier cryptosystem, which is used in various parts of the project.
        \item cryptopp-cmake: is the directory which is used by our CmakeLists.txt file to install the cryptopp library. 
    \end{itemize}
    \item \textbf{Other Scripts}:
    \begin{itemize}
        \item TestScript.sh: A key script for running customized test cases and generating experimental data. 
        \item FixingTestInstallCryptoPP.sh: A helper script to fix installation issues related to the Crypto++ library, which might be used in the project.
    \end{itemize}

\end{itemize}
This structure is designed to keep the project modular and organized, with clear separation between the core source code, tests, and third-party dependencies.

% \emph{Here, provide additional details about the general organization
% of your artifacts.  For example, provide a general roadmap to the
% files within your artifacts.  Where is the \texttt{README}?  Where are
% the source files, the datasets, the scripts for running experiments,
% etc.?  You don't need to describe every file and directory here; just
% provide a general ``lay of the land.''}

%%%%%

\subsubsection{Security, privacy, and ethical concerns}

\emph{[Mandatory]}

\textbf{Root Access Requirement}: Installing CondTypTop may require root access to the machine. This is because the installation process can involve modifying the Pluggable Authentication Module (PAM) on the system. Modifying PAM can affect how authentication is handled at the system level, which could potentially disrupt login processes if not done correctly. Users should ensure they have proper system backups before proceeding with the installation of CondTypTop, particularly on production machines.

Since CondTypTop modifies the PAM configuration, there is a risk of misconfiguration, which could lock users out of their systems or interfere with other authentication mechanisms. It is essential to follow the installation instructions carefully and, if possible, test the changes in a non-production environment.

\textbf{No Data Privacy Risks and Destructive Actions}: There are no privacy risks associated with the installation of the \textit{conditional encryption} component. The encryption schemes operate locally, and there is no transmission of sensitive data to external sources. The encryption algorithms themselves are designed to enhance security rather than pose any threats to data privacy. The execution of the conditional encryption algorithms does not involve any destructive steps, nor does it disable any security mechanisms that could expose the machine to risks. All computations are local, and no external communication is involved, minimizing security concerns.

In summary, while CondTypTop requires caution due to potential system-level modifications, the conditional encryption component poses no significant security or privacy risks. Users should ensure they understand the changes being made to their authentication modules and test carefully before applying to critical systems.
%
% \emph{Describe any risks that people might be exposed to while
% executing your artifacts: e.g., risks to their machines' security,
% data privacy, or other ethical concerns.  This is particularly
% important if destructive steps are taken or security mechanisms are
% disabled during execution.}

%%%%%

\subsubsection{How to access}
\emph{[Mandatory]}

The artifact-related data are publicly available on Zenodo with the DOI link:. The latest version of the GitHub repository, along with its corresponding link, is also provided on the Zenodo page as a commitment to ensuring access to the version of the artifact at the time of submission.

% \emph{Describe how to access your artifacts.  If your artifacts have
% received the \emph{Artifacts Available} badge, you must provide the
% DOI(s) for the permanently and publicly available copies of your
% artifacts.  Most likely, this is the version of your artifacts that
% you deposited with Zenodo.}

% \emph{You may describe more than one way to access your artifacts.
% For example, if the archived versions of your artifacts are available
% at Zenodo, and you are also making maintained versions of your
% artifacts available through GitHub, you can describe how to access
% both versions of your artifacts.}

%%%%%

\subsubsection{Hardware dependencies}

\emph{[Mandatory]}
None.
% \emph{State any specific hardware features that are required to make
% use of your artifacts: e.g., vendor, CPU/GPU/FPGA, number of
% processors/cores, microarchitecture, interconnect, memory, hardware
% counters, etc.  If your artifacts do not have significant hardware
% dependencies, simply write ``None'' in this section.}

%%%%%

\subsubsection{Software dependencies}

\emph{[Mandatory]}
The system used for this artifact runs on Ubuntu 24.04 LTS with GNOME version 46 and the Wayland windowing system. The kernel version is Linux 6.8.0-41-generic. To compile the project from source, the following software packages and dependencies are required:
\begin{itemize}
    \item[-] CMake (version 3.6 or later)
    \item[-] protobuf: Install using sudo apt install protobuf-compiler
    \item[-] PAM development library: Install using sudo apt-get install libpam0g-dev
    \item[-] cURL: Install using sudo apt install libcurl4-openssl-dev
    \item[-] Catch2: Clone the repository and build it manually
    \item[-] \textbf{cryptopp}, \textbf{zxcvbn}, and \textbf{plog}: These libraries are included in the repository and will build automatically
    \item[-] Argon2: The source for Argon2 memory-hard functions is included in the repository, but it requires manual building.
\end{itemize}
  No proprietary software is required, and all necessary open-source dependencies can either be installed via package managers or are included in the repository.

% \emph{State any specific OS and software packages that are required to
% make use of your artifacts.  This is particularly important if you
% share your source code and it must be compiled, or if your artifacts
% rely on proprietary software that is not included in your artifact
% packages.  If your artifacts do not have significant software
% dependencies, simply write ``None'' in this section.}

%%%%%

\subsubsection{Benchmarks}

\emph{[Mandatory]}

We use Chatterjee's typo correction study dataset, which is publicly available at \url{https://pages.cs.wisc.edu/~chatterjee/projects/pwtypos.html}. Specifically, we utilized the \textbf{MTurk15-General-typing.json.bz2} dataset. From this dataset, we generated various subsets by applying specific conditions, such as filtering passwords based on lengths (less than 8, 16, 32, 64, and 128 characters) and evaluating whether the Hamming distance at most T (for T = {1, 2, 3, 4}) holds. These extracted datasets were used for testing our conditional encryption algorithms in both basic functionality tests and performance evaluation experiments.

We should highlight that use these data sets for basic functionality test and evaluation of CondTypTop system as well.

% \emph{Describe any data (e.g., datasets, models, workloads,
% etc.)\ required by the experiments that are reported in your paper and
% supported by your artifacts.  If this does not apply to your
% artifacts, simply write ``None'' in this section.}

%%%%%%%%%%%%%%%%%%%%%%%%%%%%%%%%%%%%%%%%%%%%%%%%%%%%%%%%%%%%%%%%%%%%%

\subsection{Set Up}
To set up the environment for using our artifacts, you can begin by cloning the artifact repository using standard Git commands. After cloning, execute a series of basic commands to install the necessary dependencies and compile the conditional encryption schemes and the CondTypTop system. A detailed description of these steps, including the exact commands for installation, compilation, and testing, can be found in the README.md file within the repository. This process ensures that both the encryption schemes and the CondTypTop system are correctly installed and configured for use.
% \emph{This section should summarize the installation and configuration
% steps that a person should follow to prepare an environment for making
% use of your artifacts.  If the set-up steps are complicated, point the
% reader to the places in your artifacts where detailed set-up
% instructions can be found.}

%%%%%

\subsubsection{Installation-Conditional Encryption}
\emph{[Mandatory]}

 In what follows we mention the dependencies and the way to install and compile each project on your local machine.

\textbf{Dependencies}
To compile the project from source, you will need the following:
\begin{itemize}
    \item \texttt{cmake >= 3.18}
    \item \texttt{protobuf} source (in debian use sudo apt install protobuf-compiler)
    \item \texttt{pam-dev} (in debian use \texttt{sudo apt-get install libpam0g-dev})
    \item \texttt{cURL} (in debian use \texttt{sudo apt install libcurl4-openssl-dev})
    \texttt{catch2} source (to install, clone the repository and build)
    \item \texttt{cryptopp}, \texttt{zxcvbn} and \texttt{plog} (inside the repository, will automatically build)
    \item \texttt{Argon2} memory hard functions Source (inside the repository, requires manually building)
\end{itemize}

\subsubsection*{Building the Project}

\noindent \textbf{Clone the repository}
\begin{verbatim}
$ git clone https://github.com/mhassanameri/CondEncCCS24
Artifact.git
$ cd CondEncCCS24Artifact
\end{verbatim}

\noindent \textbf{Build the Argon2 libraries}
\begin{verbatim}
$ cd argon2/phcargon2
$ make
$ cd ../../
\end{verbatim}

\noindent \textbf{Create a build directory and build the program}
\begin{verbatim}
$ mkdir build && cd build
$ cmake ../
$ make
\end{verbatim}

\noindent If the \texttt{make} command fails with errors related to \texttt{g\_argvPathHint}, run the following script in the build directory, and then rerun \texttt{make}:
\begin{verbatim}
$ ../FixingTestInstallCryptoPP.sh
$ make
\end{verbatim}

\noindent Finally, to verify that the implementations of all Conditional Encryption schemes (associated with the predicates: Hamming Distance at most T, Edit Distance at most one, CAPSLOCK\_ON, and OR\_of\_CAPSLOCK\_HamDist2\_EditDist1) are working correctly, run:
\begin{verbatim}
$ ./test/tests
\end{verbatim}

The last execution runs all the test cases defined in the artifact. However, for more customized tests, such as basic tests for a specific predicate, you can use the scripts provided in the repository (which will be automatically copied to the build/test sub directory). Detailed instructions for running these basic tests are available in the "Basic Test" section of the documentation. These tests allow for focused evaluation of individual predicates, such as Hamming Distance, Edit Distance, and others, to verify their functionality in isolation. 

%%%%%

\subsubsection{Installation-CondTypTop}

\subsubsection{Basic test for Conditional Encryption}

\emph{[Mandatory]}
Instructions for Running a Simple Functionality Test
\begin{enumerate}
    \item Navigate to the Build Directory: Open a terminal and change to the directory where the build artifacts are located. This directory should contain the \texttt{TestScript.sh} file.
    \begin{verbatim}
        $ cd CondEncCCS24Artifact/build/test
    \end{verbatim}
    \item Check the Script: Open \texttt{TestScript.sh} in a text editor to review its contents. Read through the instructions and comments inside the script. This will help you understand what the script does and if any modifications are needed to initiate the desired test before executing the following command 
    \begin{verbatim}
        $ ./TestScript.sh
    \end{verbatim}
    \item  If the script requires modifications (e.g., setting input parameters, the number of test cases, target predicates, etc.), make the necessary changes and save the file after editing.

    \item Ensure that \texttt{TestScript.sh} is executable by running  
\begin{verbatim}
  $  chmod +x TestScript.sh
\end{verbatim}
This steps may be optional as we already handled it with the \texttt{CMakeLists.txt} and you can run it just in case the script is not executing after modification. 

\item Run the script: Now the script is ready to be executed to run our desired test case by the following command

\begin{verbatim}
   $ ./TestScript.sh 
\end{verbatim}

\item Verify the output: As the final step, you need to verify the generated output.  After running the script, check the output in the terminal. The expected successful output should indicate that all required software components are correctly installed and functioning as intended. This might include messages confirming successful execution of commands or proper setup.

In what follow we provide and an example of Expected Output after running the \texttt{TestScript.sh}. 
\begin{verbatim}
    $ Copy and past one example of success full 
    execution from terminal. 
\end{verbatim}

\end{enumerate}

\subsubsection{Basic test for CondTypTop}\hassan{Will be added. }

% \emph{Provide instructions for running a simple functionality test.
% This test does not need to exercise all the features of your
% artifacts, but ideally, it should allow a user to check that all of
% the required software components are correctly installed and
% functioning as intended.  Please include the expected successful
% output and any required input parameters.}

%%%%%%%%%%%%%%%%%%%%%%%%%%%%%%%%%%%%%%%%%%%%%%%%%%%%%%%%%%%%%%%%%%%%%

\subsection{Evaluation Workflow}

\emph{This section should include all the operational steps and
experiments that a person must be carry out to utilize in your
artifacts toward the goal of validating your paper's key results and
claims.  To that end, we ask you to use the two following subsections
and cross-reference the items therein as explained below.}

%%%%%

\subsubsection{Major claims}

\emph{[Mandatory for \emph{Artifacts Evaluated--Functional},
  \emph{Artifacts Evaluated--Reusable}, and \emph{Results Reproduced};
  optional for \emph{Artifacts Available}]}
\emph{Enumerate here the major claims (Cx) made in your paper.  Follow
the examples below.}
\bigskip

\begin{itemize}

\item[(C1):]
  \emph{System\_name achieves the same accuracy as the
  state-of-the-art systems for a task X while requiring Y\% less
  storage.  This is proven by the experiment (E1) described in [refer
    to your paper's sections], whose results are illustrated/reported
  in [refer to your paper's plots, tables, sections, etc.].}

\item[(C2):]
  \emph{System\_name has been used to uncover new bugs in the X
  software.  This is proven by experiments (E2) and (E3) in [refer to
    your paper's sections].}
\end{itemize}

%%%%%

\subsubsection{Experiments}

\emph{[Mandatory for \emph{Artifacts Evaluated--Functional},
  \emph{Artifacts Evaluated--Reusable}, and \emph{Results Reproduced};
  optional for \emph{Artifacts Available}]}
\emph{Explicitly link the descriptions of your experiments to the
items you have provided in the previous subsection about major claims.
Please provide estimates of the person- and compute-time required for
each of the listed experiments (using the suggested hardware/software
configuration).  Follow the examples below.}

\bigskip
\begin{itemize}
\item[(E1):]
  \emph{[Optional Name] [30~person-minutes + 1~compute-hour + 5\,GB
    disk]: Provide a short explanation of the experiment and expected
  results.}

  \emph{Provide the steps to perform the experiment and collect and
  organize the results as expected from your paper.  We encourage you
  to use the following structure with three main blocks for the
  description of your experiment.  If the procedures are complicated,
  point the reader to the places in your artifacts where the full
  instructions can be found.}

  \begin{itemize}
  \item[Preparation:] \emph{Describe the steps required to prepare and
  configure the environment for this experiment.}

  \item[Execution:] \emph{Describe the steps required to run this
  experiment.}

  \item[Results:] \emph{Describe the steps required to collect and
  interpret the results for this experiment.}
  \end{itemize}

\item[(E2):] \emph{[Optional Name] [1~person-hour + 3~compute-hours]: \ldots}

\item[(E3):] \emph{[Optional Name] [1~person-hour + 3~compute-hours]: \ldots}
\end{itemize}
\bigskip

\emph{In all of the above blocks, please provide indications about the
expected outcome for each of the steps (given the suggested hardware
and software configuration).}

%%%%%%%%%%%%%%%%%%%%%%%%%%%%%%%%%%%%%%%%%%%%%%%%%%%%%%%%%%%%%%%%%%%%%

\subsection{Notes on Reusability}

\emph{[Optional]}
\emph{This section is meant to provide additional information about
how a person could utilize your artifacts beyond the research
presented in your paper.  A broad objective of artifact evaluation is
to encourage you to make your research artifacts reusable by others.}

\emph{Include in this section any instructions, guidance, or advice
that you believe would help others reuse your artifacts.  For example,
you could describe how one might scale certain components of your
artifacts up or down; apply your artifacts to different kinds of
inputs or datasets; customize your artifacts' behavior by replacing
specific modules or algorithms; etc.}

%%%%%%%%%%%%%%%%%%%%%%%%%%%%%%%%%%%%%%%%%%%%%%%%%%%%%%%%%%%%%%%%%%%%%

\subsection{Version}
%%%%%%%%%%%%%%%%%%%%
% Obligatory.
% Do not change/remove.
%%%%%%%%%%%%%%%%%%%%
Based on the LaTeX template for Artifact Evaluation V20220926.

%%%%%%%%%%%%%%%%%%%%%%%%%%%%%%%%%%%%%%%%%%%%%%%%%%%%%%%%%%%%%%%%%%%%%

%% AUTHORSHIP AND PROVENANCE OF THIS TEMPLATE

%% This template was created by Eric Eide for the ACM CCS 2024
%% conference.
%%
%% The AEC Chair for CCS 2024 was:
%% Eric Eide (University of Utah)

%% This template is based on the "USENIX Security 2023 AE Template."
%% https://secartifacts.github.io/usenixsec2023/appendix/usesec23-ae-latex.zip
%%
%% The AEC Co-chairs for USENIX Security 2023 were:
%% Cristiano Giuffrida (Vrije Universiteit Amsterdam)
%% Anjo Vahldiek-Oberwagner (Intel Labs)

%% The USENIX Security AE template was based on the
%% % Artifact Appendix Template for EuroSys'22 AE
%% https://sysartifacts.github.io/eurosys2022/appendix/EuroSys22_ArtifactAppendix_template.tex
%%
%% The AEC Co-chairs for EuroSys 2022 were:
%% Natacha Crooks (UC Berkeley)
%% Solal Pirelli (EPFL)
%% Salvatore Signorello (University of Lisbon)
%% Anjo Vahldiek-Oberwagner (Intel Labs)

%% The above were based on:

%% LaTeX template for Artifact Evaluation V20220119
%%
%% Original Authors
%% * Grigori Fursin (cTuning foundation, France) 2014-2020
%% * Bruce Childers (University of Pittsburgh, USA) 2014
%%
%% Modified by
%% * Clementine Maurice (CNRS, France) 2021-2022
%% * Cristiano Giuffrida (Vrije Universiteit Amsterdam, Netherlands) 2021-2022
%%
%% (C) Copyright 2014-2022
%%
%% CC BY 4.0 license
%%
